# Supplementary material for: Dispersive nodal fermions along grain boundaries in Floquet topological crystals
Source: arXiv:2212.08060 ancillary file (2025-01-14)
Supplement: Supplementary file 1 [file Supplementary_GrainBoundary.pdf]

# Supplemental Material: Dynamic metal along grain boundaries in Floquet topological crystals

Daniel J. Salib<sup>1</sup> and Bitan Roy<sup>1</sup>

<sup>1</sup>*Department of Physics, Lehigh University, Bethlehem, Pennsylvania, 18015, USA*

(Dated: December 15, 2022)

In this Supplemental Material, we present (a) additional details on the grain boundary physics for the static Chern insulator [Sec. S1 and Fig. S1], (b) details of the Floquet unitary operator and the effective Floquet Hamiltonian for kick, step and sinusoidal drives [Sec. S2], and (c) dynamic metallic states along the large angle grain boundaries stemming from these three types of time periodic drives [Sec. S3 and Figs. S2-S4].

## S1. STATIC CHERN INSULATOR AND LARGE ANGLE GRAIN BOUDANRY

In the main manuscript we argue that in the parameter regime  $-2 < m_0/t_0 < 0$  the static Hamiltonian  $H_{\text{stat}}$  displays band inversion at the M point of the Brillouin zone [see Eq. (1) of the main text]. This can be anchored by computing the one-dimensional (1D) band structure of  $H_{\text{stat}}$  with  $k_x$  as a conserved quantity and an open boundary condition along the  $y$  direction. As shown in Fig. S1(a), such a band structure manifests edge modes crossing the zero energy at momentum  $k_x = \pi$  (projection of the M point). Then the  $\mathbf{K} \cdot \mathbf{b}$  rule indicates that for  $\mathbf{K}_{\text{inv}} = (\pi, \pi)/a$  and  $\mathbf{b} = \pm a\hat{\mathbf{e}}_1$ ,  $\Phi_{\text{dis}} = \pi$  (nontrivial) and even large angle grain boundaries host robust 1D metallic states along such line defects, as can be seen from the energy spectra of the corresponding Hamiltonian [Fig. S1(b)] as well as from the local density of states (LDOS) of these modes, which is highly localized along the grain-antigrain boundary pair [Fig. S1(c)]. Furthermore, a Fourier transformation of the same set of states as a function of the conserved momentum  $k_y$  (since  $\mathbf{b} = \pm a\hat{\mathbf{e}}_1$  in our construction) anchor their metallic or gapless nature [Fig. S1(d)].

## S2. FLOQUET UNITARY OPERATOR AND EFFECTIVE FLOQUET HAMILTONIAN

This section is devoted to the discussion on the unitary Floquet time evolution operator and the corresponding effective Hamiltonian for the kick, step and sinusoidal drives. We discuss these three cases separately next.

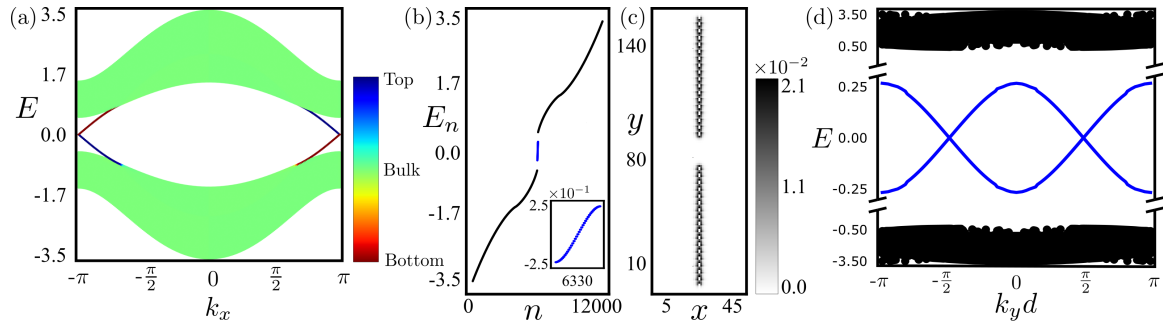

Figure S1. Static Chern insulator and large angle grain boundaries therein. (a) One-dimensional band structure of  $H_{\text{stat}}$  [see Eq. (1) of the main text] for  $t = t_0 = 1$  and  $m_0 = -1.5$ , yielding the translationally active M phase featuring band inversion at the M point of the Brillouin zone, and resulting in edge modes crossing the zero energy at  $k_x = \pm\pi$ . The system size in the  $y$  direction with open boundary condition (OBC) is 100. (b) The energy spectra of  $H_{\text{stat}}$  in a periodic system with a grain-antigrain boundary pair each containing 18 (anti)dislocations, with the Burgers vector  $\mathbf{b} = \pm a\hat{\mathbf{e}}_1$  for the same parameters as in (a), supporting one-dimensional metallic states (blue dots in the inset) along the line defects around zero energy. (c) The local density of states of these modes show high localization along the line defects. (d) A Fourier transformation of the same set of states as a function of the conserved momentum  $k_y$  confirms their metallic nature.

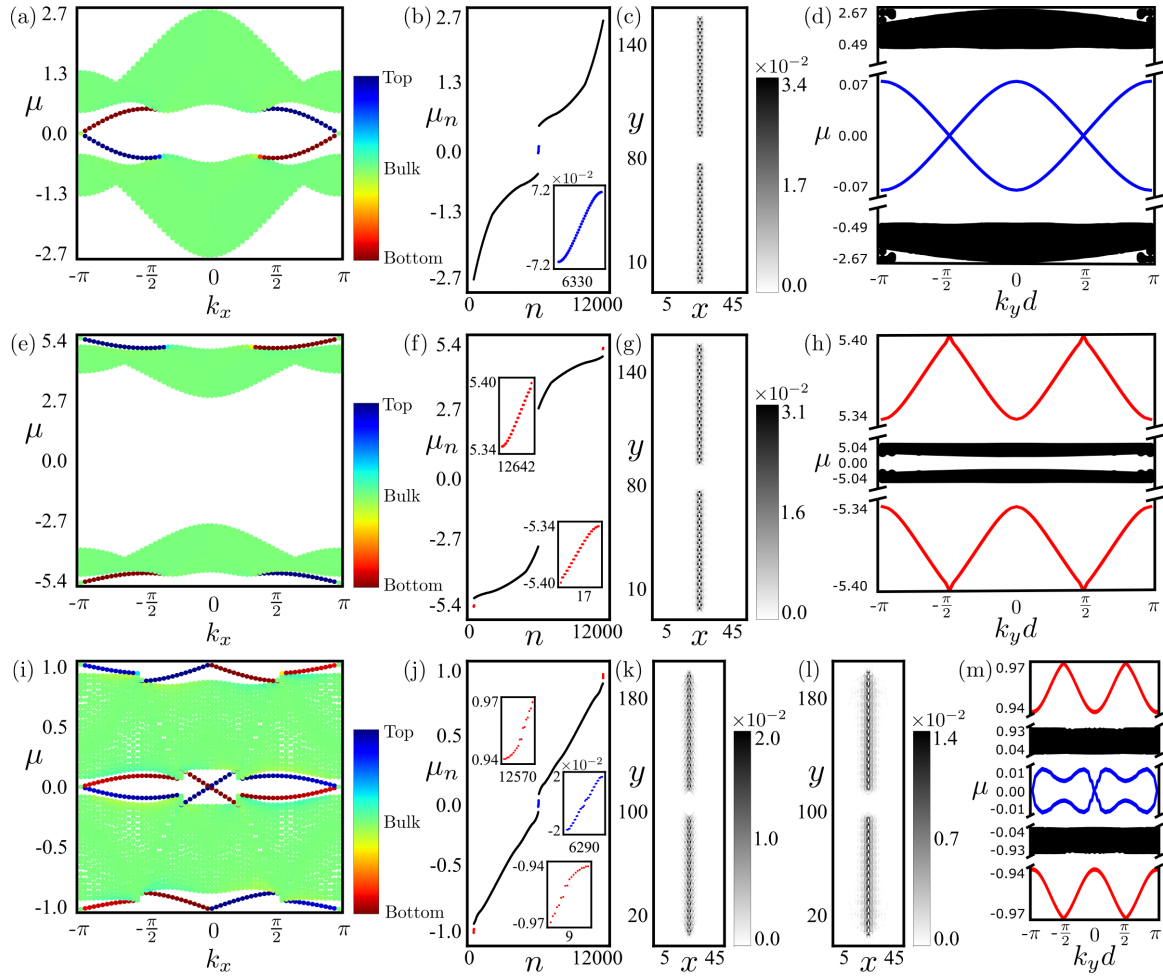

Figure S2. Driven time reversal odd insulators and large angle grain boundaries therein in the presence of a kick drive [see Eq. (4) of the main text]. (a) One-dimensional band structure in terms of quasienergies of the eigenmodes of the unitary time evolution operator  $U(k_x, T)$  [see Eq. (7) of the main text] at the stroboscopic time  $T = 2\pi/\omega$  for  $\omega = 12.8$  and  $m_1 = -1.8$ , yielding Floquet-Bloch band inversion at the M point of the Floquet Brillouin zone center, resulting in edge modes crossing the zero quasienergy at  $k_x = \pm\pi$ . Here the system size in the  $y$  direction with OBC is 60. (b) Quasienergy spectra of  $U(T)$  in a system with periodic boundary condition and a pair of grain-antigrain boundary each containing 18 (anti)dislocations, with the Burgers vector  $\mathbf{b} = \pm a\hat{\mathbf{e}}_1$  for the same parameters as in (a), supporting one-dimensional dynamic normal metallic states (blue dots in the inset) along the line defects, as shown through their local density of states (LDOS) in (c). (d) Fourier transformation of these states as a function of the conserved momentum  $k_y$  confirms their metallic nature. Panels (e)-(h) are similar to (a)-(d), respectively, but for  $\omega = 10.8$ ,  $m_1 = -5.2$  giving rise to edge modes crossing quasienergies  $\pm\omega/2$  at  $k_x = \pm\pi$  (resulting from the inversion of the Floquet-Bloch bands at the Floquet zone boundaries) and an anomalous dynamic metal (red dots) near the Floquet zone boundaries. Panels (i) and (j) are similar to (a) and (b), respectively, but for  $\omega = 1.94$  and  $m_1 = -4.5$ , yielding edge modes crossing the zero and  $\pm\omega/2$  quasienergies. Edge modes near  $k_x = 0$  and  $\pm\pi$  (either at the center or boundaries of the Floquet zone) result from the Floquet-Bloch band inversion at the  $\Gamma$  and M points, respectively. The former does not give rise to any defect modes as then  $\mathbf{K}_{\text{inv}}^{\text{Flq}} \cdot \mathbf{b} = 0$ . The system supports a mixed dynamic metal simultaneously hosting normal and anomalous dynamic metals. Their LDOS are respectively shown in (k) and (l). (m) Fourier transformation of these states confirms their metallicity near both Floquet zone center and boundaries. Throughout, we set  $t = t_0 = 1$  and  $m_0 = 3.0$ .

For the kick drive [see Eq. (4) of the main text], the unitary time evolution operator takes the following form

$$U(\mathbf{k}, T) = \text{TO} \left( \exp \left[ -i \int_0^T [H_{\text{stat}} + V(t)] dt \right] \right) = \exp(-im_1\tau_3) \exp(-iH_{\text{stat}}T) \equiv \exp(-iTH_{\text{Flq}}(\mathbf{k})).$$

The effective Floquet Hamiltonian  $H_{\text{Flq}}(\mathbf{k}) = \boldsymbol{\tau} \cdot \mathbf{d}_{\text{Flq}}(\mathbf{k}, T)$ , where  $\boldsymbol{\tau} = (\tau_1, \tau_2, \tau_3)$  is the vector Pauli matrix and

$\mathbf{d}_{\text{Flq}}(\mathbf{k}, T) = (d_{1,\text{Flq}}(\mathbf{k}), d_{2,\text{Flq}}(\mathbf{k}), d_{3,\text{Flq}}(\mathbf{k}))$  with

$$\begin{aligned} d_{1,\text{Flq}}(\mathbf{k}) &= \frac{d_0}{\sin(d_0 T)} \left( B \frac{d_1(\mathbf{k})}{|\mathbf{d}(\mathbf{k})|} - D \frac{d_2(\mathbf{k})}{|\mathbf{d}(\mathbf{k})|} \right), & d_{2,\text{Flq}}(\mathbf{k}) &= \frac{d_0}{\sin(d_0 T)} \left( B \frac{d_2(\mathbf{k})}{|\mathbf{d}(\mathbf{k})|} + D \frac{d_1(\mathbf{k})}{|\mathbf{d}(\mathbf{k})|} \right), \\ d_{3,\text{Flq}}(\mathbf{k}) &= \frac{d_0}{\sin(d_0 T)} \left( B \frac{d_3(\mathbf{k})}{|\mathbf{d}(\mathbf{k})|} + C \right), & \text{with } d_0(\mathbf{k}) &= \frac{1}{T} \arccos \left( A - D \frac{d_3(\mathbf{k})}{|\mathbf{d}(\mathbf{k})|} \right), \end{aligned} \quad (\text{S1})$$

and

$$A = \cos(|\mathbf{d}(\mathbf{k})T|) \cos m_1, \quad B = \sin(|\mathbf{d}(\mathbf{k})T|) \cos m_1, \quad C = \cos(|\mathbf{d}(\mathbf{k})T|) \sin m_1, \quad D = \sin(|\mathbf{d}(\mathbf{k})T|) \sin m_1. \quad (\text{S2})$$

For the step drive [see Eq. (5) of the main text], the  $d$ -vector can be expressed in an effective time-dependent form

$$\mathbf{d}_{\text{eff}}(\mathbf{k}, t) = \begin{cases} \mathbf{d}_1(\mathbf{k}) & nT < t < nT + T/4 \\ \mathbf{d}_2(\mathbf{k}) & nT + T/4 < t < nT + 3T/4, \\ \mathbf{d}_3(\mathbf{k}) & nT + 3T/4 < t < (n+1)T \end{cases} \quad (\text{S3})$$

where  $\mathbf{d}_\mu(\mathbf{k}) = (d_1(\mathbf{k}), d_2(\mathbf{k}), d_3(\mathbf{k}) + m_\mu)$ . Let us introduce  $\theta_\mu = |\mathbf{d}_\mu(\mathbf{k})| \Delta T_\mu$ , where  $\Delta T_1 = \Delta T_3 = T/4$  and  $\Delta T_2 = T/2$ . Then the time evolution operator for the step drive at the stroboscopic time reads

$$U(\mathbf{k}, T) = \text{TO} \left( \prod_{j=1}^3 \exp \left[ -i \theta_j \frac{\mathbf{d}_j(\mathbf{k})}{|\mathbf{d}_j(\mathbf{k})|} \cdot \boldsymbol{\tau} \right] \right) = \text{TO} \left( \prod_{j=1}^3 \left[ \cos \theta_j - i \sin \theta_j \frac{\mathbf{d}_j(\mathbf{k})}{|\mathbf{d}_j(\mathbf{k})|} \cdot \boldsymbol{\tau} \right] \right).$$

In what follows  $i, j$ , and  $k$  are related with the cyclic permutation  $i \rightarrow j \rightarrow k \rightarrow i$  and  $i, j, k = 1, 2, 3$ . Next we define the following quantities

$$\begin{aligned} \alpha &= \prod_{i=1}^3 \cos \theta_i, \quad \beta = \prod_{i=1}^3 \frac{\sin \theta_i}{|\mathbf{d}_i(\mathbf{k})|}, \quad A_i = \frac{\cos \theta_i \sin \theta_j \sin \theta_k}{|\mathbf{d}_j(\mathbf{k})| |\mathbf{d}_k(\mathbf{k})|}, \quad B_i = \frac{\sin \theta_i \cos \theta_j \cos \theta_k}{|\mathbf{d}_i(\mathbf{k})|}, \quad Q_i = \mathbf{d}_j(\mathbf{k}) \cdot \mathbf{d}_k(\mathbf{k}), \\ R_i &= (-1)^{i+1} d_2(\mathbf{k})(m_j - m_k), \quad S_i = (-1)^i d_1(\mathbf{k})(m_j - m_k), \quad \zeta_0 = \alpha - \sum_{i=1}^3 A_i Q_i, \\ \zeta_1 &= \sum_{i=1}^3 A_i R_i + d_1(\mathbf{k}) \sum_{i=1}^3 B_i - \beta [Q_3 d_1(\mathbf{k}) + S_3 (d_3(\mathbf{k}) + m_3)], \\ \zeta_2 &= \sum_{i=1}^3 A_i S_i + d_2(\mathbf{k}) \sum_{i=1}^3 B_i - \beta [Q_3 d_2(\mathbf{k}) - R_3 (d_3(\mathbf{k}) + m_3)], \quad \zeta_3 = \sum_{i=1}^3 B_i (d_3(\mathbf{k}) + m_i) - \beta [R_3 d_2(\mathbf{k}) + Q_3 (d_3(\mathbf{k}) + m_3)]. \end{aligned} \quad (\text{S4})$$

The effective Floquet Hamiltonian is expressed in terms of

$$\mathbf{d}_{\text{Flq}}(\mathbf{k}) = d_0(\mathbf{k}) \mathbf{d}'(\mathbf{k}) = d_0(\mathbf{k}) (d'_1(\mathbf{k}), d'_2(\mathbf{k}), d'_3(\mathbf{k})), \quad (\text{S5})$$

where

$$d_0(\mathbf{k}) = \frac{1}{T} \arccos \zeta_0 \quad \text{and} \quad d'_\mu(\mathbf{k}) = \frac{d_0}{\sin(d_0 T)} \zeta_\mu \quad \text{for } \mu = 1, 2, 3. \quad (\text{S6})$$

For the sinusoidal drive [see Eq. (6) of the main manuscript], the time integration appearing in the time evolution operator can be approximated in the large  $N$  limit as

$$\int_0^t [H_{\text{stat}} + V \cos(\omega t') \tau_3] dt' \approx \sum_{j=0}^{N-1} [H_{\text{stat}} + V \cos(\omega t_j) \tau_3] \delta t, \quad (\text{S7})$$

where  $t_j = (j + 1/2)\delta t$  and  $\delta t = t/N$ . With this approximation, the time evolution operator takes the form

$$U(\mathbf{k}, t) = \prod_{j=0}^{N-1} \exp [-i (H_{\text{stat}} + V \cos(\omega t_j) \tau_3) \delta t] = \prod_{j=0}^{N-1} U(\mathbf{k}, t_j + \delta t) U(\mathbf{k}, t_j). \quad (\text{S8})$$

The time evolution from  $t_j$  to  $t_j + \delta t$  can be approximated using the Trotter-Suzuki decomposition, which is accurate for  $\delta t \ll t$ , yielding

$$U(\mathbf{k}, t_j + \delta t) U(\mathbf{k}, t_j) \approx \exp \left( -i \frac{\delta t}{2} V \cos(\omega t_j) \tau_3 \right) \exp (-i \delta t H_{\text{stat}}) \exp \left( -i \frac{\delta t}{2} V \cos(\omega t_j) \tau_3 \right). \quad (\text{S9})$$

For a sinusoidal drive,  $\mathbf{d}_{\text{Flq}}(\mathbf{k})$  cannot be written in a compact analytic form. We compute it numerically.

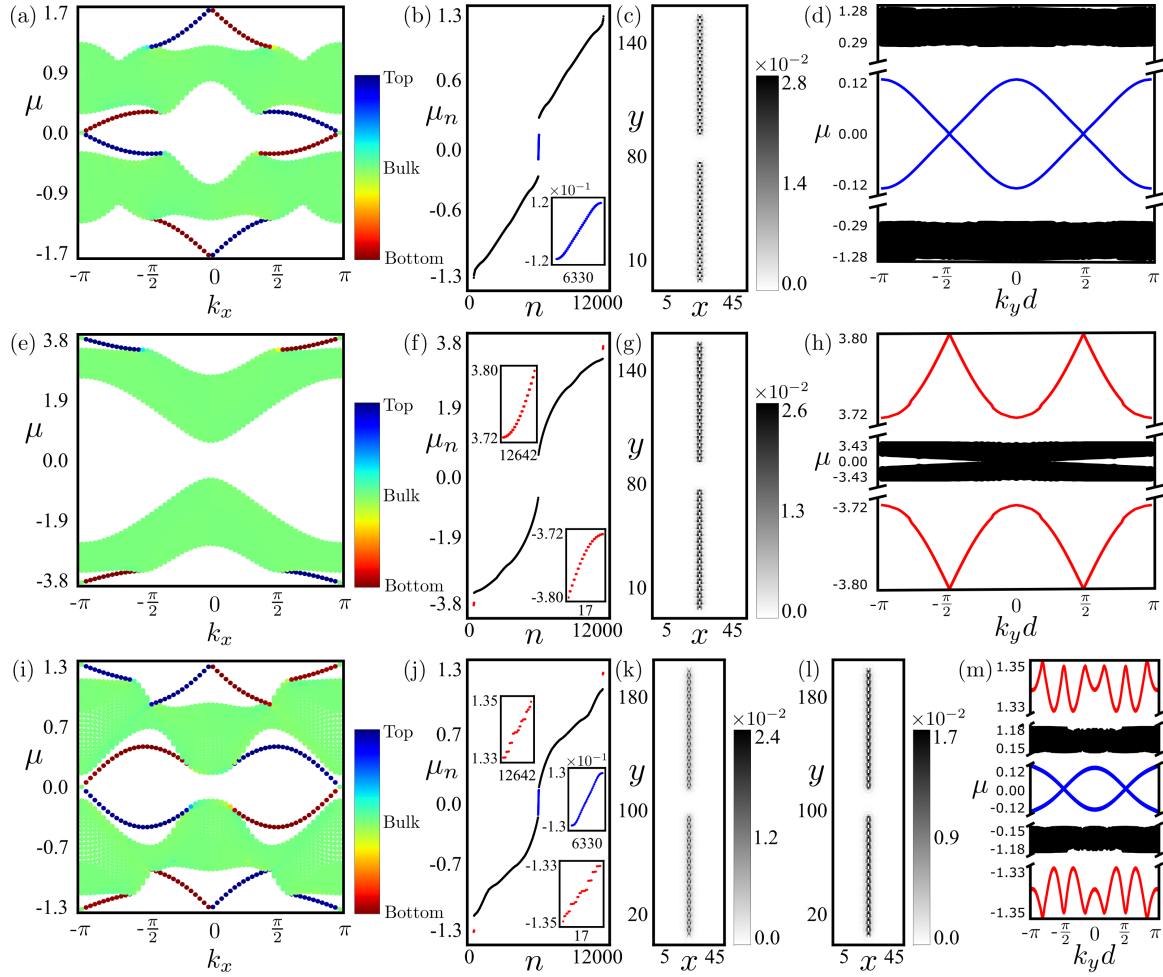

Figure S3. Driven time reversal odd insulators and large angle grain boundaries therein in the presence of a step drive [see Eq. (5) of the main text]. (a) One-dimensional band structure in terms of quasienergies of the eigenmodes of the unitary time evolution operator  $U(k_x, T)$  [see Eq. (7) of the main text] at the stroboscopic time  $T = 2\pi/\omega$  for  $\omega = 3.5$  and  $m_2 = -2.5$ , yielding Floquet-Bloch band inversion at the M point of the Floquet Brillouin zone center, resulting in edge modes crossing the zero quasienergy at  $k_x = \pm\pi$ . Here the system size in the  $y$  direction with OBC is 60. (b) Quasienergy spectra of  $U(T)$  in a system with periodic boundary condition and a pair of grain-antigrain boundary each containing 18 (anti)dislocations, with the Burgers vector  $\mathbf{b} = \pm a\hat{\mathbf{e}}_1$  for the same parameters as in (a), supporting one-dimensional dynamic normal metallic states (blue dots in the inset) along the line defects, as shown through their local density of states (LDOS) in (c). (d) Fourier transformation of these states as a function of the conserved momentum  $k_y$  confirms their metallic nature. Panels (e)-(h) are similar to (a)-(d), respectively, but for  $\omega = 7.6$ ,  $m_2 = -2.8$  giving rise to edge modes crossing quasienergies  $\pm\omega/2$  at  $k_x = \pm\pi$  (resulting from the inversion of the Floquet-Bloch bands at the Floquet zone boundaries) and an anomalous dynamic metal (red dots) near the Floquet zone boundaries. Panels (i) and (j) are similar to (a) and (b), respectively, but for  $\omega = 2.7$  and  $m_2 = -2.9$ , yielding edge modes crossing  $\pm\omega/2$  quasienergies at  $k_x = \pm\pi$ . The system supports a mixed dynamic metal simultaneously hosting normal and anomalous dynamic metals. Their LDOS are respectively shown in (k) and (l). (m) Fourier transformation of these states confirms their metallicity near both Floquet zone center and boundaries. In (a) and (i), we also find edge modes crossing  $\pm\omega/2$  quasienergies at  $k_x = 0$  due to Floquet-Bloch band inversion at the  $\Gamma$  point at the Floquet zone boundaries. However, they do not lead to any metallic state at the grain-antigrain boundary pair as  $\mathbf{K}_{\text{inv}}^{\text{Flq}} \cdot \mathbf{b} = 0$  for these states. Throughout, we set  $t = t_0 = 1$ ,  $m_1 = m_3 = 2$  and  $m_0 = 3.0$ .

### S3. ADDITIONAL NUMERICAL RESULTS

In this section, we present additional numerical results in favor of the dynamic generation of 1D topological metallic states along the grain boundary, which we claim to be insensitive to the drive protocol. In the main manuscript, we anchored this outcome for small angle grain boundaries, characterized by the angle  $\theta = 11.54^\circ < 15^\circ$ . Here we

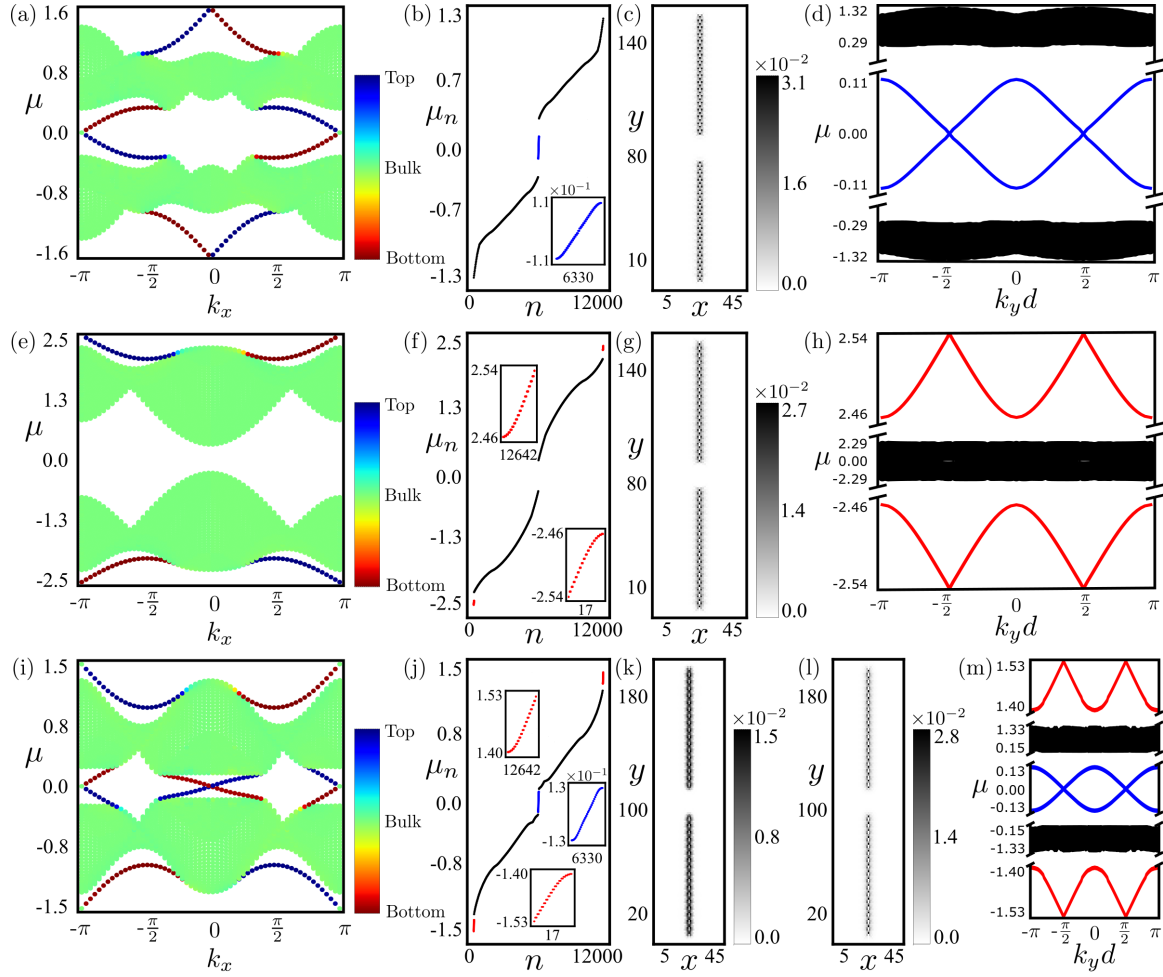

Figure S4. Driven time reversal odd insulators and large angle grain boundaries therein in the presence of a sinusoidal drive [see Eq. (6) of the main text]. (a) One-dimensional band structure in terms of quasienergies of the eigenmodes of the unitary time evolution operator  $U(k_x, T)$  [see Eq. (7) of the main text] at the stroboscopic time  $T = 2\pi/\omega$  for  $\omega = 3.1$  and  $m_0 = 2.42$ , yielding Floquet-Bloch band inversion at the M point of the Floquet Brillouin zone center, resulting in edge modes crossing the zero quasienergy at  $k_x = \pm\pi$ . Here the system size in the  $y$  direction with OBC is 60. (b) Quasienergy spectra of  $U(T)$  in a system with periodic boundary condition and a pair of grain-antigrain boundary each containing 18 (anti)dislocations, with the Burgers vector  $\mathbf{b} = \pm a\hat{\mathbf{e}}_1$  for the same parameters as in (a), supporting one-dimensional dynamic normal metallic states (blue dots in the inset) along the line defects, as shown through their local density of states (LDOS) in (c). (d) Fourier transformation of these states as a function of the conserved momentum  $k_y$  confirms their metallic nature. Panels (e)-(h) are similar to (a)-(d), respectively, but for  $\omega = 5.08$ ,  $m_0 = -2.79$  giving rise to edge modes crossing quasienergies  $\pm\omega/2$  at  $k_x = \pm\pi$  (resulting from the inversion of the Floquet-Bloch bands at the Floquet zone boundaries) and an anomalous dynamic metal (red dots) near the Floquet zone boundaries. Panels (i) and (j) are similar to (a) and (b), respectively, but for  $\omega = 3.06$  and  $m_2 = 1.33$ , yielding edge modes crossing the zero and  $\pm\omega/2$  quasienergies at  $k_x = \pm\pi$ . The system supports a mixed dynamic metal simultaneously hosting normal and anomalous dynamic metals. Their LDOS are respectively shown in (k) and (l). (m) Fourier transformation of these states confirms their metallicity near both Floquet zone center and boundaries. In (a) and (i), we also find edge modes crossing  $\pm\omega/2$  and zero quasienergies at  $k_x = 0$  due to Floquet-Bloch band inversion at the  $\Gamma$  point at the Floquet zone boundaries and center, respectively. However, they do not lead to any metallic state at the grain-antigrain boundary pair as  $\mathbf{K}_{\text{inv}}^{\text{Flq}} \cdot \mathbf{b} = 0$  for these states. Throughout, we set  $t = t_0 = 1$  and  $V = 3.0$ .

show that the same conclusion qualitatively holds also for the large angle grain boundary. We now set  $d = 2a$ , where  $d$  is the separation between the cores of two neighboring (anti)dislocations and  $a$  is the lattice spacing, yielding  $\theta = 30^\circ > 15^\circ$ . For all three drive protocols we choose the same parameter values used in the main manuscript. Then the effective 1D band structure of the unitary Floquet time evolution operator displays edge modes crossing zero and  $\pm\omega/2$  quasienergies at  $k_x = \pm\pi$  whenever we find 1D normal and anomalous metallic states along the grain boundary, respectively. Similarly, when the system supports a mixed 1D metal along such a 1D line defect, the edge

modes cross the zero and  $\pm\omega/2$  quasienergies at  $k_x = \pm\pi$  simultaneously. These results are shown in Fig. S2, Fig. S3 and Fig. S4 for the kick, step and sinusoidal drives, respectively.

For a large angle grain-antigrain boundary pair, the system then supports 1D dynamic metallic states along such line defects near the Floquet zone center (normal metal), Floquet zone boundaries (anomalous metal) as well as Floquet zone center and boundaries (mixed metal). We arrive at these conclusions by computing the quasienergy spectra for the associated unitary time evolution operator, the local density of states of the in-gap quasimodes localized near the Floquet zone center and/or boundaries, as well their Fourier transformations in term of the conserved momentum  $k_y$ .
